# Supplementary material for: On the Intrinsic Self-Correction Capability of LLMs: Uncertainty and Latent Concept
Source: arXiv:2406.02378 source file (2024-11-07)
Supplement: Supplementary file 1 [file social_impact.tex]

\section{Broader Impact \label{app: broader}}
Our paper focuses on the self-correction capability of LLMs, which helps mitigate harmful, toxic, and biased behaviors, resulting in a positive social impact. 
Our work demonstrates that proper instruction design can enhance the effectiveness of self-correction, ensuring the reliability of LLMs without the risk of failure.
% , indicating the reliability of the self-correction capability of LLM without failure potential. 
We do not foresee any negative broader impacts stemming from our findings. We expect our work to significantly contribute to the ongoing research efforts aimed at enhancing the self-correction capability and broadening the usage of LLMs across more diverse tasks.
